# Supplementary material for: Policy Learning for Optimal Dynamic Treatment Regimes with Observational Data
Source: arXiv:2404.00221 source file (2026-11-28)
Supplement: Supplementary file 2 [file table_simulation_supplement.tex]

\begin{table}[htbp]
\centering
\caption{Monte Carlo simulation results for DGP1 with Missspecification}
\label{table:simulatin_results_dgp1_miss}
\bigskip
\scalebox{0.9}{
\begin{tabular}{cccccccc}
\hline
\multicolumn{1}{c}{} & \multicolumn{2}{c}{Specification} & \multicolumn{5}{c}{Sample Size} \\
\cmidrule(l{3pt}r{3pt}){2-3} \cmidrule(l{3pt}r{3pt}){4-8}
Method & Q-function & PS & 250 & 500 & 1000 & 2000 & 4000 \\
\hline
\multirow{2}{*}{Q-learn} 
    & correct & -     & 0.20 (0.12) & 0.31 (0.11) & 0.43 (0.10) & 0.57 (0.07) & 0.68 (0.03) \\
    & miss    & -     & 0.25 (0.09) & 0.28 (0.07) & 0.31 (0.05) & 0.33 (0.04) & 0.33 (0.03) \\ \hdashline
\multirow{2}{*}{Q-search} 
    & correct & -     & 0.17 (0.19) & 0.29 (0.21) & 0.40 (0.21) & 0.53 (0.16) & 0.64 (0.10) \\
    & miss    & -     & 0.23 (0.16) & 0.23 (0.16) & 0.23 (0.16) & 0.22 (0.16) & 0.18 (0.15) \\ \hdashline
\multirow{2}{*}{IPW} 
    & -       & correct & 0.24 (0.13) & 0.29 (0.14) & 0.37 (0.16) & 0.45 (0.14) & 0.55 (0.13) \\
    & -       & miss    & 0.24 (0.11) & 0.29 (0.12) & 0.32 (0.12) & 0.39 (0.13) & 0.44 (0.14) \\ \hdashline
\multirow{3}{*}{DR} 
    & correct & miss    & 0.24 (0.14) & 0.37 (0.16) & 0.54 (0.15) & 0.67 (0.08) & 0.72 (0.03) \\
    & miss    & correct & 0.34 (0.17) & 0.46 (0.15) & 0.59 (0.11) & 0.67 (0.04) & 0.69 (0.03) \\
    & correct & correct & 0.29 (0.17) & 0.44 (0.17) & 0.61 (0.11) & 0.70 (0.04) & 0.72 (0.02) \\
\hline
\end{tabular}

}
\smallskip
\begin{tablenotes} \footnotesize
\item Notes: The columns labeled ``Specification'' indicate the specifications of the Q-functions and propensity scores (PS), respectively, where ``correct'' and ``miss'' refer to correct specification and misspecification. Each cell in the last five columns reports the mean welfare, with the standard deviation in parentheses, for each method, specification, and sample size. These values are calculated based on 500 simulations using a test sample of 50,000 observations randomly drawn from DGP1.
\end{tablenotes} 
\end{table}

\begin{table}[htbp]
\centering
\caption{Monte Carlo simulation results for DGP2 with Missspecification}
\label{table:simulatin_results_dgp2_miss}
\bigskip
\scalebox{0.9}{
\begin{tabular}{cccccccc}
\hline
\multicolumn{1}{c}{} & \multicolumn{2}{c}{Specification} & \multicolumn{5}{c}{Sample Size} \\
\cmidrule(l{3pt}r{3pt}){2-3} \cmidrule(l{3pt}r{3pt}){4-8}
Method & Q-function & PS & 250 & 500 & 1000 & 2000 & 4000 \\
\hline
\multirow{2}{*}{Q-learn} 
    & correct & -     & 1.31 (0.36) & 1.69 (0.11) & 1.78 (0.08) & 1.84 (0.05) & 1.89 (0.05) \\
    & miss    & -     & 1.46 (0.07) & 1.50 (0.05) & 1.52 (0.04) & 1.53 (0.03) & 1.54 (0.03) \\ \hdashline
\multirow{2}{*}{Q-search} 
    & correct & -     & 1.26 (0.48) & 1.58 (0.18) & 1.54 (0.09) & 1.52 (0.04) & 1.54 (0.04) \\
    & miss    & -     & 1.44 (0.15) & 1.44 (0.12) & 1.44 (0.10) & 1.43 (0.08) & 1.42 (0.08) \\ \hdashline
\multirow{2}{*}{IPW} 
    & -       & correct & 1.30 (0.21) & 1.42 (0.17) & 1.56 (0.19) & 1.68 (0.21) & 1.81 (0.21) \\
    & -       & miss    & 1.32 (0.18) & 1.41 (0.13) & 1.49 (0.10) & 1.51 (0.07) & 1.52 (0.07) \\ \hdashline
\multirow{3}{*}{DR} 
    & correct & miss    & 1.44 (0.21) & 1.63 (0.23) & 1.78 (0.22) & 1.87 (0.19) & 1.99 (0.19) \\
    & miss    & correct & 1.56 (0.23) & 1.69 (0.25) & 1.85 (0.23) & 1.95 (0.16) & 2.02 (0.16) \\
    & correct & correct & 1.51 (0.26) & 1.77 (0.24) & 1.95 (0.14) & 2.01 (0.07) & 2.04 (0.07) \\
\hline
\end{tabular}

}
\smallskip
\begin{tablenotes} \footnotesize
\item Notes: The columns labeled ``Specification'' indicate the specifications of the Q-functions and propensity scores (PS), respectively, where ``correct'' and ``miss'' refer to correct specification and misspecification. Each cell in the last five columns reports the mean welfare, with the standard deviation in parentheses, for each method, specification, and sample size. These values are calculated based on 500 simulations using a test sample of 50,000 observations randomly drawn from DGP2.
\end{tablenotes} 
\end{table}
